# Supplementary material for: Knowing When to Stop: Efficient Context Processing via Latent Sufficiency Signals
Source: arXiv:2502.01025 source file (2026-10-09)
Supplement: Supplementary file 4 [file algo.tex]

% \section{Dynamic Context Cutoff Algorithm} 
% \label{app:algo}
% \begin{algorithm}[h]
% \caption{\textbf{Dynamic Context Cutoff}}
% \begin{algorithmic}[1]
% \REQUIRE Pre-trained Language Model $\mathcal{M}$ \\
% Input query $q$ \\
% Full context $\mathbf{C}$, partitioned into $m$ contiguous segments $\{\mathfrak{s}_j\}_{j=1}^m$ \\
% Sufficiency classifier $\mathcal{S}$ with confidence function $\mathcal{S}_c(\cdot)$ \\
% Threshold $\tau$

% \ENSURE 
%  Minimal sufficient prefix $\mathbf{C}_k$ s.t. $\mathcal{M}(q,\mathbf{C}_k) \approx \mathcal{M}(q,\mathbf{C})$

% \STATE \textbf{Initialize:} 
% \STATE \quad $\mathbf{C}_1 \gets \mathfrak{s}_1$ \quad \textit{/* first chunk */}
% \STATE \quad $\mathbf{A}_{\text{cache}}^0 \gets \varnothing$ \quad \textit{/* empty cache */}

% \FOR{$i = 1$ \textbf{to}  $m$}
%     \STATE \textit{// Process only the newly added segment $\mathfrak{s}_i$ on top of the cached activations}
%     \STATE $\mathbf{A}(\mathbf{C}_i) \gets f_{\text{model}}\bigl(\mathfrak{s}_i,\mathbf{A}_{\text{cache}}^{i-1}\bigr)$
%     \STATE \textit{// Update the cache with new activations}
%     \STATE $\mathbf{A}_{\text{cache}}^{i} \gets \mathbf{A}_{\text{cache}}^{i-1} \cup \mathbf{A}(\mathbf{C}_i)$

%     \STATE \textit{// Compute classifier confidence for sufficiency}
%     \STATE $s \gets \mathcal{S}_c(\mathbf{C}_i)$

%     \IF{$s \ge \tau$}
%         \STATE \textbf{return} $\mathbf{C}_i$ \quad \textit{/* Early stop: $\mathbf{C}_i$ is sufficient */}
%     \ENDIF

%     \STATE \textit{// If not sufficient, extend the prefix}
%     \IF{$i < m$}
%        \STATE $\mathbf{C}_{i+1} \gets \mathbf{C}_{i} \mathbin\Vert \mathfrak{s}_{i+1}$
%        \quad \textit{/* Prepare next chunk */}
%     \ENDIF
% \ENDFOR

% \STATE \textbf{return} $\mathbf{C}_m$
% \quad \textit{/* If no early stop, use entire context */}

% \end{algorithmic}
% \end{algorithm}
