# Supplementary material for: Knowing When to Stop: Efficient Context Processing via Latent Sufficiency Signals
Source: arXiv:2502.01025 source file (2026-10-09)
Supplement: Supplementary file 5 [file baselines.tex]

\section{Baselines}
\label{app:baselines}
\rx{
todo: add a brief description of the each baselines. provide math formula for each. }
\pr{

The baselines used in the paper are:

\begin{enumerate}
    \item \textbf{BM25 (RAG)} – A term-frequency-based retrieval algorithm that selects the most relevant context chunks for processing.
    \item \textbf{SBERT (RAG)} – Uses a transformer-based sentence encoder to retrieve the most semantically relevant context chunks.
    \item \textbf{LLMLingua (Compression)} – A token-level compression approach that removes low-entropy tokens using perplexity scores.
    \item \textbf{LongLLMLingua (Compression)} – An extension of LLMLingua for long-context scenarios, using hierarchical, question-aware filtering.
    \item \textbf{LLMLingua2 (Compression)} – A task-agnostic prompt compression method that distills knowledge from a large LLM into a smaller token classifier.
    \item \textbf{Supervised Fine-Tuning (SFT)} – A fine-tuned model trained to predict sufficiency and stop processing when enough information is gathered.
    \item \textbf{Self-Prompting} – Uses the LLM's own response to a self-assessment prompt to determine when to stop processing.
\end{enumerate}

}
\paragraph{Random}
