# Supplementary material for: Knowing When to Stop: Efficient Context Processing via Latent Sufficiency Signals
Source: arXiv:2502.01025 source file (2026-10-09)
Supplement: Supplementary file 7 [file evaluation.tex]

\section{Evaluation Metrics}
\label{app:evaluation}
\rx{todo - discussion on why we use these metrics, why not flops (no suprising that less context requires less flop - show a graph), why not stander F1/EM for QA - folloing previous work that evals QA using model-based \cite{helmet}, which is more accurate especially for long context.}
