# Supplementary material for: Knowing When to Stop: Efficient Context Processing via Latent Sufficiency Signals
Source: arXiv:2502.01025 source file (2026-10-09)
Supplement: Supplementary file 9 [file model.tex]

\section{Model Selection} 
\label{app:models}
To ensure a comprehensive evaluation, we selected models from three popular families: LLaMA, Qwen, and Mistral. These models were chosen to cover a wide range of parameter scales (1B to 70B), ensuring the evaluation spans lightweight to high-capacity setups. Priority was given to instruction-tuned variants, as they align better with user-centric tasks such as question answering. The selection ensures the our method’s generalizability across architectures and parameter sizes.
