# Supplementary material for: Knowing When to Stop: Efficient Context Processing via Latent Sufficiency Signals
Source: arXiv:2502.01025 source file (2026-10-09)
Supplement: Supplementary file 11 [file recall_precision.tex]

\section{Recall at High Precision}
\label{app:recall_precision}

\begin{figure}[ht!]
    \centering
    %\vspace{-2mm}
    \includegraphics[width=.5\linewidth]{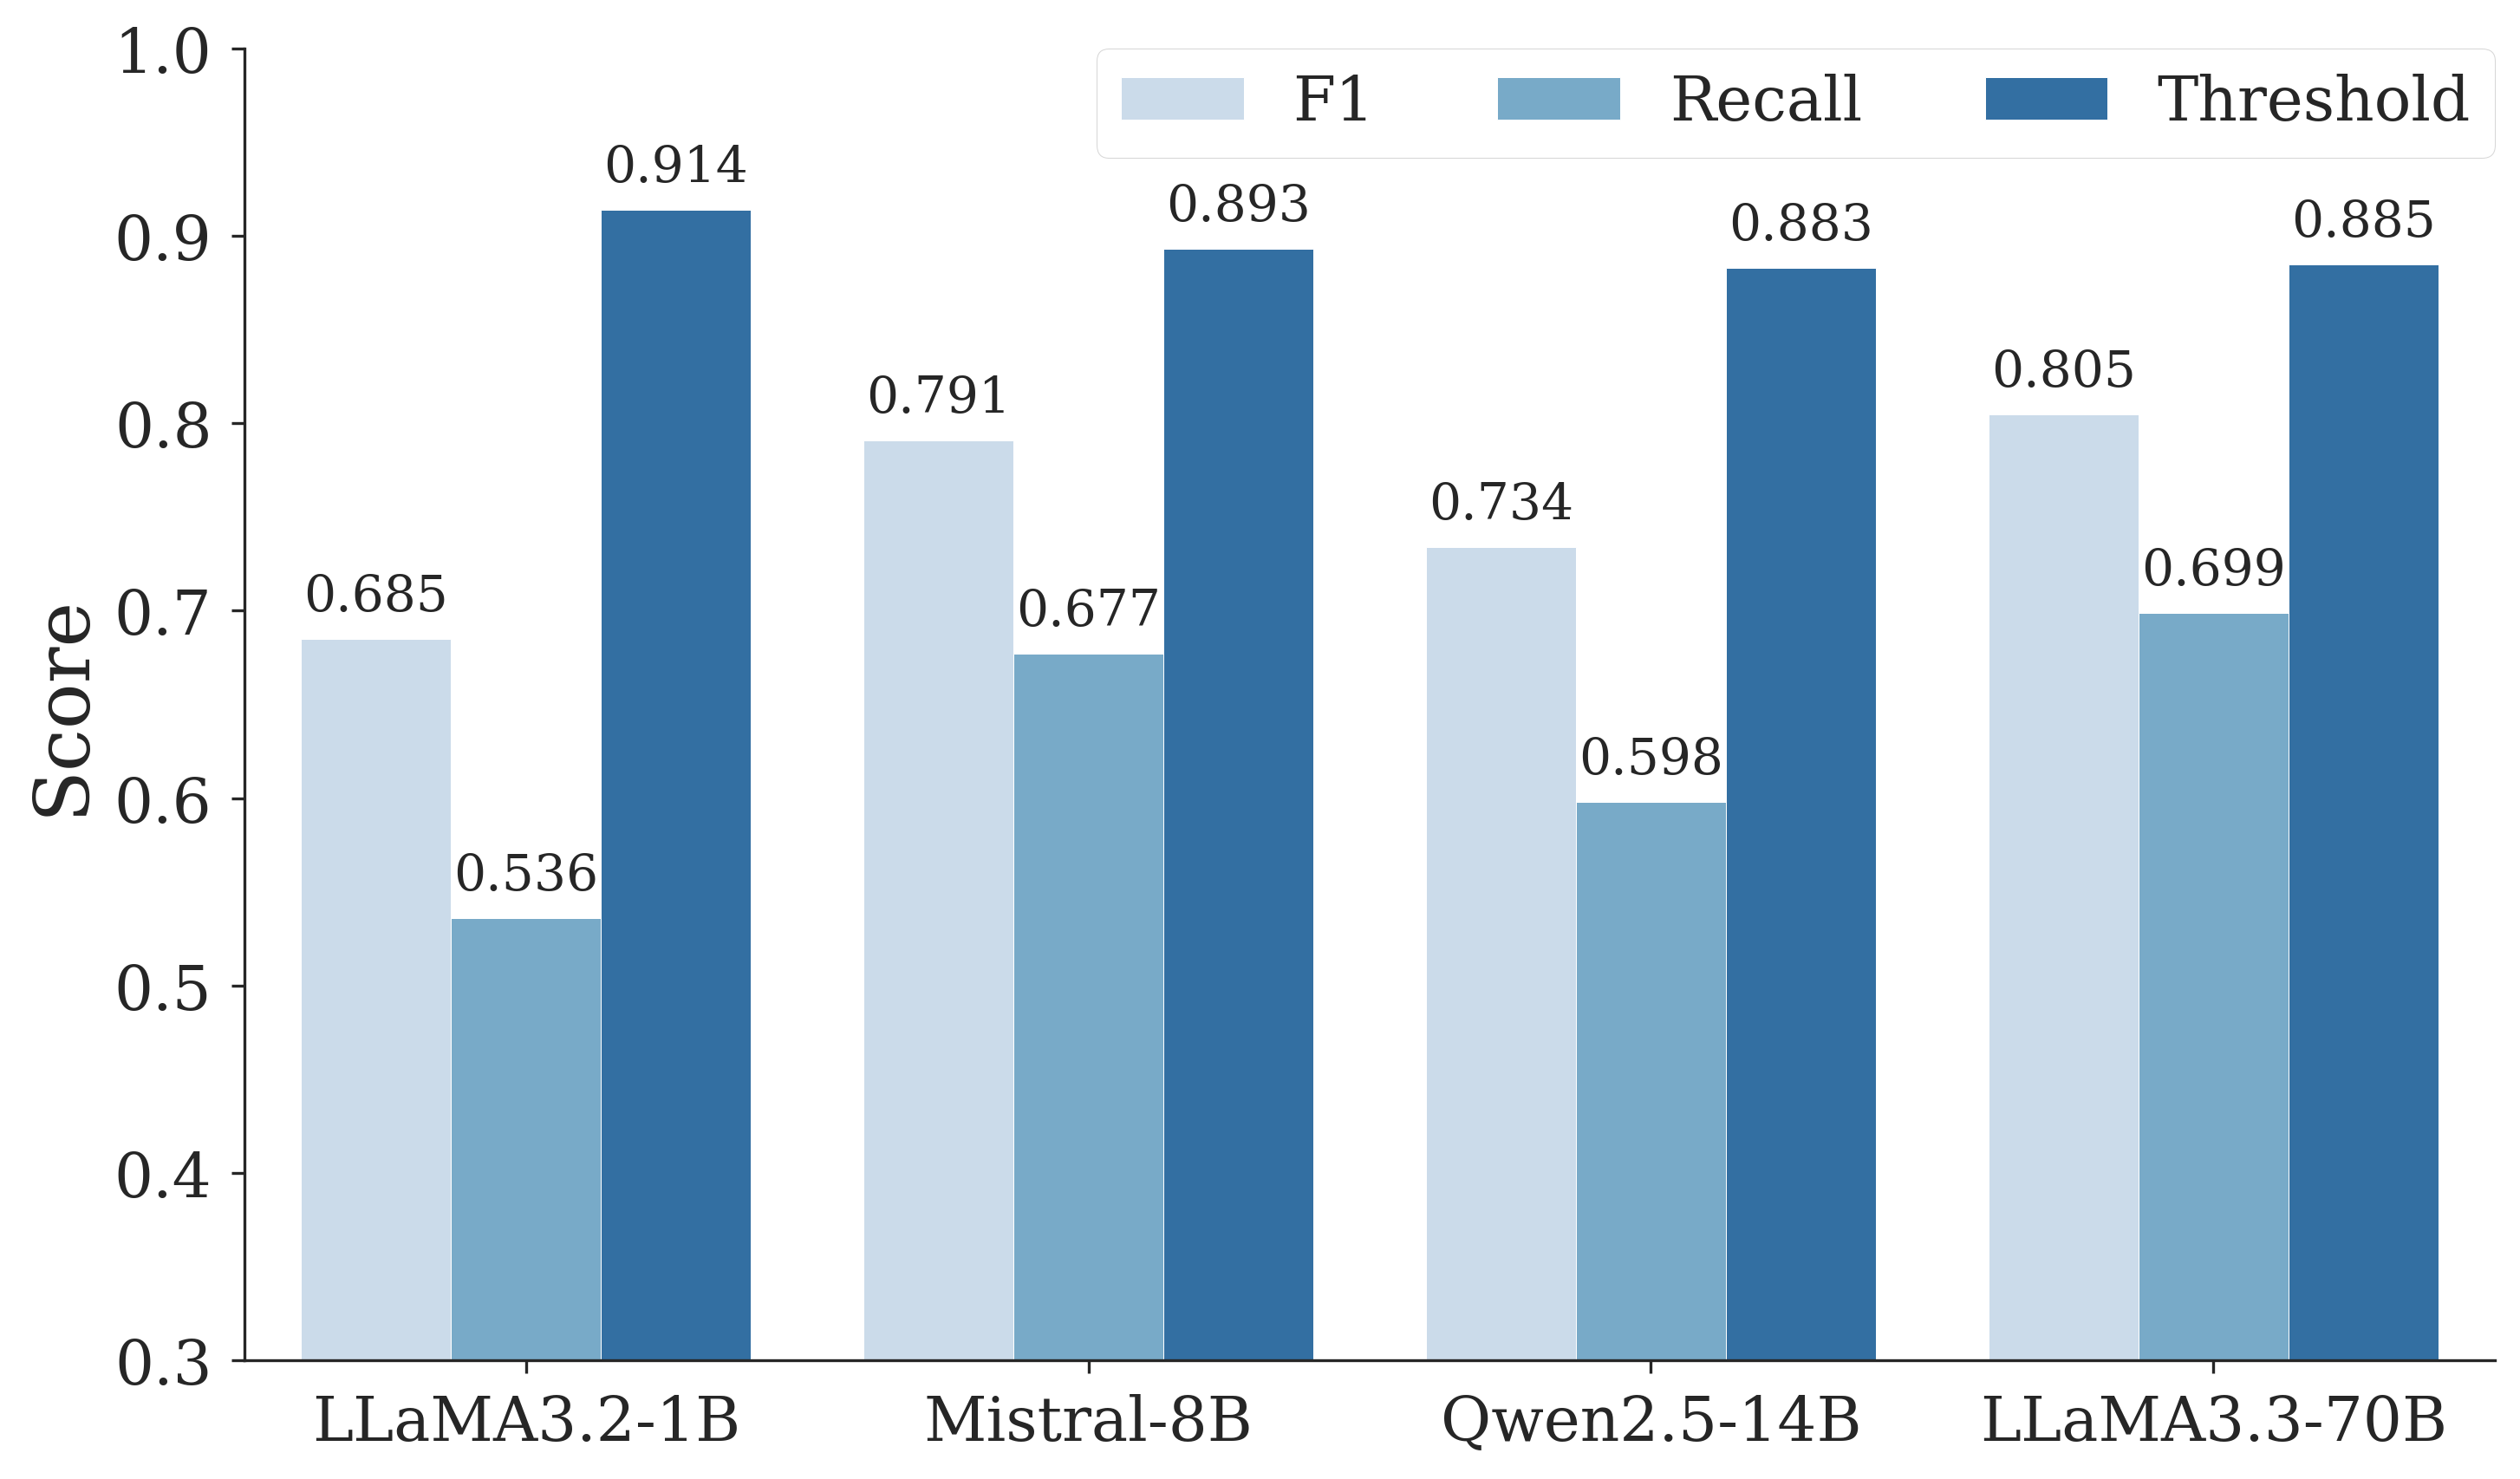}
    %\vspace{-6mm}
    \caption{F1 score and Recall at 95\% precision (R@95P) for sufficiency detection.}
   % \vspace{-6mm}
    \label{fig:confidence_trends}
    \end{figure}

\begin{figure}[ht!]
    \centering
    %\vspace{-2mm}
    \includegraphics[width=.5\linewidth]{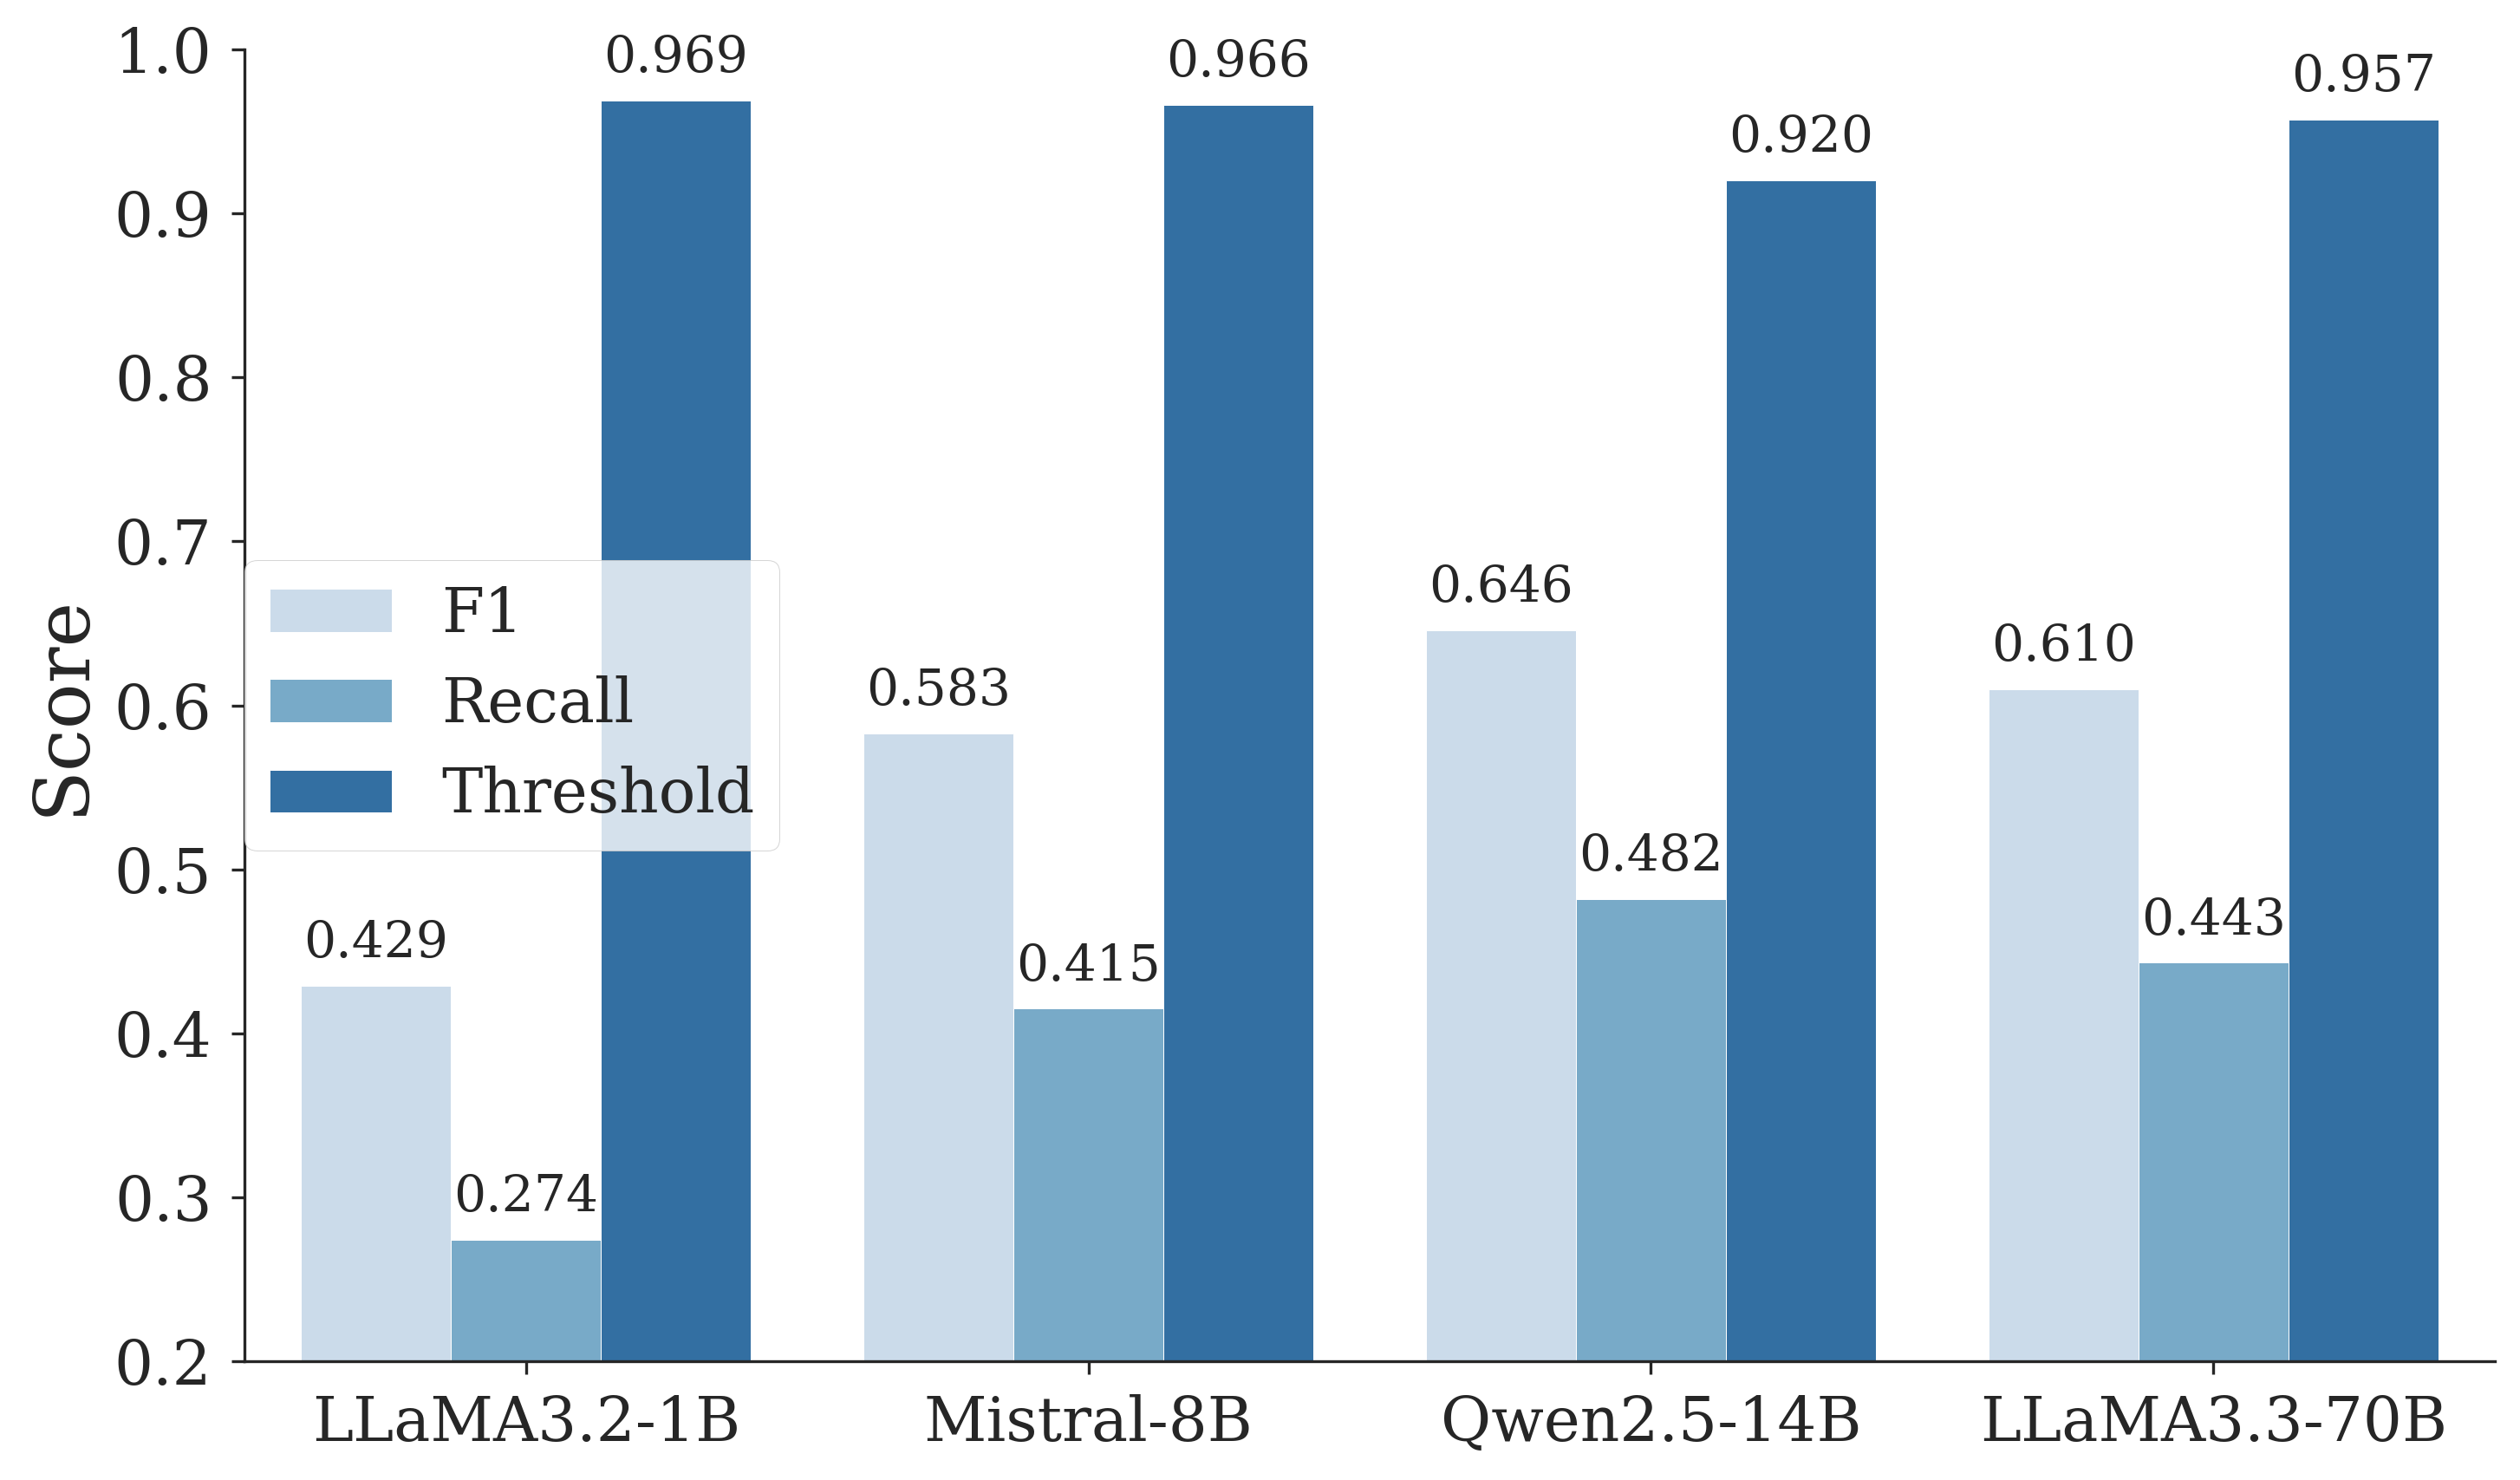}
    %\vspace{-6mm}
    \caption{F1 score and Recall at 98\% precision (R@98P) for sufficiency detection.}

   % \vspace{-6mm}
    \label{fig:confidence_trends}
    \end{figure}

% \begin{figure}[t!]
%     \centering
%      \begin{subfigure}[b]{0.45\textwidth}
%         \centering
%         \includegraphics[width=\linewidth]{figures/p95_metrics.png}
%         \caption{F1 score and Recall at 95\% precision (R@95P) for sufficiency detection.}
%         \label{fig:f1_p95}
%     \end{subfigure}
%     \hfill
%     \begin{subfigure}[b]{0.45\textwidth}
%         \centering
%         \includegraphics[width=\linewidth]{figures/p98_metrics.png}
%         \caption{F1 score and Recall at 98\% precision (R@98P) for sufficiency detection.}
%         \label{fig:f1_p98}
%     \end{subfigure}
%     \vspace{-4mm}
%     \caption{ }
%     \vspace{-2mm}
%     \label{fig:f1_combined}
% \end{figure}

% \begin{figure}[t!]
% \centering
% % \vspace{-2mm}
% \includegraphics[width=.5\linewidth]{figures/confidence_trends.png}
% %\vspace{-6mm}
% \caption{confidence vs. number of chunks: as more chunks are processed, the model's confi}
% %\vspace{-2mm}
% \label{fig:confidence_trends}
% \end{figure}
